# Supplementary material for: Flow Computation in Temporal Interaction Networks
Source: arXiv:2003.01974 source file (2020-03-04)
Supplement: Supplementary file 1 [file Appendix.tex]

\section{Appendix}\label{sec:appendix}
